# Supplementary material for: ASQ-IT: Interactive Explanations for Reinforcement-Learning Agents
Source: arXiv:2301.09941 source file (2023-01-24)
Supplement: Supplementary file 1 [file Supplementary.tex]

\appendix

\section{User Study 1: Usability Assessment}
Figure \ref{fig: M2Q} denotes an example M2Q question. The start state (top) depicts the agent in lane 1, above a blue car and the end state shows the agent below a blue car, in lane 2. All multiple-choice answers have a specification that is plausible given these two states, and only the constraint specification dictates the correct answer.

\begin{figure}
	\centering
    \frame{\includegraphics[width=0.8\columnwidth]{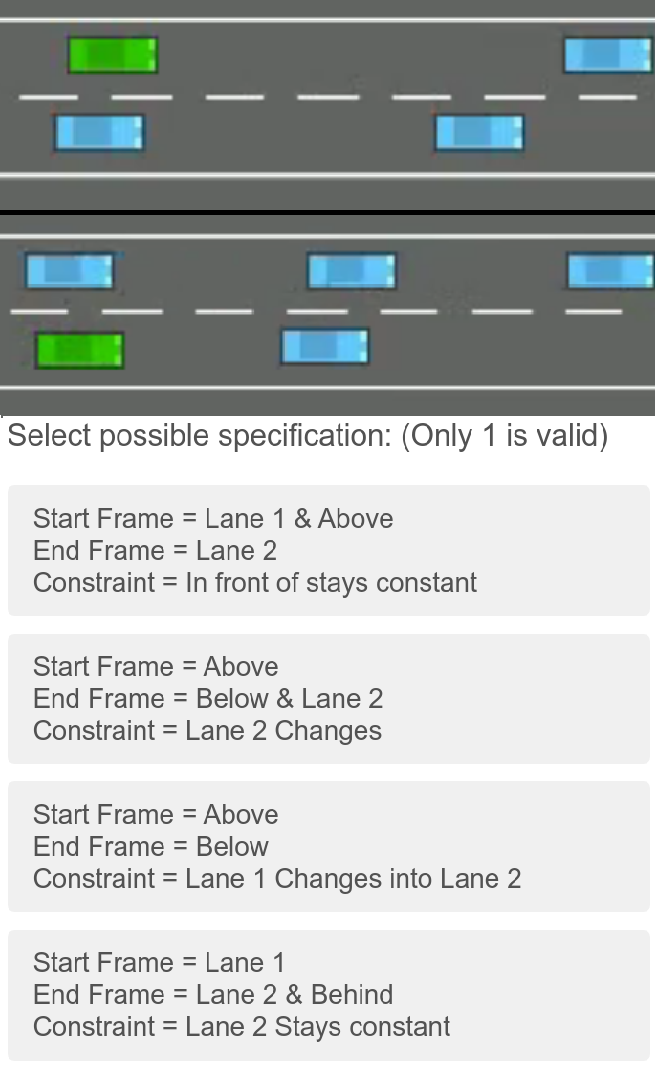}}\\
    \caption{Movie to Query (M2Q) task, question 2.\\ \textbf{Top}: Start State; \textbf{Mid}: End State; \textbf{Bottom}: Multiple Choice. \\ Full Video: \url{https://bit.ly/3GJV394}}
	\label{fig: M2Q}
\end{figure}
